# Supplementary material for: Role of enviromental dynamic polarizability in static excited state properties of embedded molecular systems: Application to disordered fluorographene systems
Source: arXiv:1808.02399 ancillary file (2018-08-07)
Supplement: Supplementary file 1 [file SupportingInformation.pdf]

# Role of enviromental dynamic polarizability in static excited state properties of embedded molecular systems: Supporting Information

*Vladislav Sláma*[1], *Frank Müh*[2], *Thomas Renger*[2], *and Tomáš Mančal*[1]

[1]Faculty of Mathematics and Physics, Charles University, Ke Karlovu 5, 121 16, Prague 2, Czech Republic
[2]Institut für Theoretische Physik, Johannes Kepler University Linz, Altenberger Str. 69, 4040 Linz, Austria

## 1 Approximations

In this section, we discuss approximations needed to obtain compact notation for the first and the second order correction to the energy shift, transition dipole and interaction energy.

First we assume that the electric field from environment charges, where only single environment building block is excited, is approximately the same as for all environment blocks in the ground state $\sum_n \frac{q_n(0,0)(r-R_n)}{|R_n-r|^3} \gg \frac{(q_{n'}(\eta,\eta)-q_{n'}(0,0))(r-R_{n'})}{|R_{n'}-r|^3}$. This is true for larger distances from the excited environment building block or when the excited state charges of the environment building blocks are similar to the ground state charges.

For interaction energies between individual excited building blocks, we use multipole expansion. The lowest nonzero contribution results in interaction between corresponding transition dipoles as $\langle\eta_n|\,\langle 0_{n'}|\,V_{nn'}\,|0_n\rangle\,|\eta'_{n'}\rangle = \vec{\mu}^{(n)}_{0\eta}\vec{\mu}^{(n')}_{0\eta'}/R^3_{nn'} - 3\left(\vec{\mu}^{(n)}_{0\eta}R_{nn'}\right)\left(\vec{\mu}^{(n')}_{0\eta'}R_{nn'}\right)/R^5_{nn'}$. The interaction between excited states of environment building blocks is therefore treated in point dipole approximation.

The crucial approximation is based on separation of sums of the type

$$\sum_\eta\sum_{\eta'}\frac{\left(\mu^{(n)}_{0\eta}\mu^{(n)}_{0\eta}\right)\left(\mu^{(n')}_{0\eta'}\mu^{(n')}_{0\eta'}\right)}{\left(F^{(n)}_{0\eta}+F^{(n')}_{0\eta'}\right)\left(F^{(n')}_{0\eta'}-E\right)} = \sum_\eta\sum_{\eta'}\frac{\left(\mu^{(n)}_{0\eta}\mu^{(n)}_{0\eta}\right)\left(\mu^{(n')}_{0\eta'}\mu^{(n')}_{0\eta'}\right)}{2F^{(n)}_{0\eta}\left(F^{(n')}_{0\eta'}-E\right)}\frac{1}{\left(1+\frac{F^{(n')}_{0\eta'}-F^{(n)}_{0\eta}}{2F^{(n)}_{0\eta}}\right)}$$

$$\approx \frac{1}{2}\sum_\eta\frac{\left(\mu^{(n)}_{0\eta}\mu^{(n)}_{0\eta}\right)}{F^{(n)}_{0\eta}}\sum_{\eta'}\frac{\left(\mu^{(n')}_{0\eta'}\mu^{(n')}_{0\eta'}\right)}{\left(F^{(n')}_{0\eta'}-E\right)}$$

$$+\frac{1}{4}\left[\sum_\eta\frac{\left(\mu^{(n)}_{0\eta}\mu^{(n)}_{0\eta}\right)}{F^{(n)}_{0\eta}}\sum_{\eta'}\frac{\left(\mu^{(n')}_{0\eta'}\mu^{(n')}_{0\eta'}\right)}{F^{(n')}_{0\eta'}} - \sum_\eta\frac{\left(\mu^{(n)}_{0\eta}\mu^{(n)}_{0\eta}\right)\sum_{\eta'}\left(\mu^{(n')}_{0\eta'}\mu^{(n')}_{0\eta'}\right)}{\left(F^{(n)}_{0\eta}\right)^2}\right]+\dots, \qquad (1)$$

where Taylor expansion was used for the cross term $\left(1+\frac{F^{(n')}_{0\eta'}-F^{(n)}_{0\eta}}{2F^{(n)}_{0\eta}}\right)^{-1}$. When the environmental block is approximated by harmonic oscillator, only transitions which differ by one qunatum number

are allowed. This results in a contribution only from the leading term of the Taylor expansion. The same is true for hydrogen-like atom for $E = 0$. We therefore adopt this assumption for our model and use

$$\sum_{\eta}\sum_{\eta'}\frac{\left(\mu_{0\eta}^{(n)}\mu_{0\eta}^{(n)}\right)\left(\mu_{0\eta'}^{(n')}\mu_{0\eta'}^{(n')}\right)}{\left(F_{0\eta}^{(n)}+F_{0\eta'}^{(n')}\right)\left(F_{0\eta'}^{(n')}-E\right)}\approx\frac{1}{2}\sum_{\eta}\frac{\left(\mu_{0\eta}^{(n)}\mu_{0\eta}^{(n)}\right)}{F_{0\eta}^{(n)}}\sum_{\eta'}\frac{\left(\mu_{0\eta'}^{(n')}\mu_{0\eta'}^{(n')}\right)}{\left(F_{0\eta'}^{(n')}-E\right)}.$$

Due to the large size of the environment, standard QC methods cannot be used for calculation of excited state charegs of the environmet. Therefore, the electrostatic interaction of the excited building block with the rest of the environment building blocks in the ground state, needs to be approximated as

$$\begin{aligned}\sum_{n'}\langle 0_{n'}|\langle\eta_n|V_{nn'}|\eta_n\rangle|0_{n'}\rangle &= \sum_{n'}\frac{q_{n'}(0,0)\left(q_n(\eta,\eta)-q_n(0,0)\right)}{R_{nn'}}+\sum_{n'}\frac{q_{n'}(0,0)\,q_n(0,0)}{R_{nn'}}\\ &= K_{\eta}^{(n)}+\sum_{n'}\frac{q_{n'}(0,0)\,q_n(0,0)}{R_{nn'}}\approx\bar{K}+\sum_{n'}\frac{q_{n'}(0,0)\,q_n(0,0)}{R_{nn'}}.\end{aligned}$$

We assume that the interaction of the single excited environment building block with the other building blocks in the ground states, is the same for every environmental building block. This approximation holds for the homogeneous environment or for the environment building blocks, where the charge distribution does not change upon the excitation (where $\bar{K} = 0$).

The last term, which needs to be approximated, is the interaction involving excitation of already excited building block, such as:

$$\begin{aligned}&\langle e0|V|g\eta_n\rangle\langle g\eta_n|V|g\eta_n'\rangle\langle g\eta_n'|V|e0\rangle\\ &=\langle A_e|\langle 0|V|\eta_n\rangle|A_g\rangle\langle A_g|\langle\eta_n|V|\eta_n'\rangle|A_g\rangle\langle A_g|\langle\eta_n'|V|0\rangle|A_e\rangle\\ &=\sum_{n'}\mathcal{E}_{ge}^{(A)}\left(R^{(n)}\right)\mu_{0\eta}^{(n)}\left[\mu_{\eta\eta'}^{(n)}\frac{(R_{n'}-R_n)}{|R_{n'}-R_n|^3}q_{n'}\right]\mu_{0\eta'}^{(n)}\mathcal{E}_{ge}^{(A)}\left(R^{(n)}\right)\approx 0.\end{aligned}$$

For hydrogen-like atoms, the transition dipole is nonzero only between states which differ in orbital quantum number $l$ by one ($\Delta l = \pm 1$). Both states $\eta$ and $\eta'$ must, due to the $\mu_{0\eta}^{(n)}$ and $\mu_{0\eta'}^{(n)}$, have the same orbital quantum number. Therefore there is a zero transition dipole moment between these states $\mu_{\eta\eta'}^{(n)}$, because $\Delta l = 0$. The same is true also for the harmonic oscillator approximation. For our model, we also adopt this assumption and neglect these contributions.

## 1.1 Excitation energy shift

When we use the approximations specified above, the second order correction to the transition energy reads as

$$
\begin{aligned}
E^{(2)}_{g\to e} \approx{}& \frac{1}{2}\left[E^{pol,2}_{ee,ee}\left(\alpha\left(0\right)\right)-E^{pol,2}_{gg,gg}\left(\alpha\left(0\right)\right)\right]+\left[E^{env-pol,2}_{ee}\left(\alpha\left(0\right)\right)-E^{env-pol,2}_{gg}\left(\alpha\left(0\right)\right)\right]\\
&+\frac{1}{4}\left[E^{pol,2}_{ge,ge}\left(\alpha\left(\varepsilon_{ge}\right)\right)+E^{pol2}_{ge,ge}\left(\alpha\left(0\right),\alpha\left(\varepsilon^{(A)}_{ge}\right)\right)\right]-\frac{1}{4}\left[E^{pol,2}_{ge,ge}\left(\alpha\left(-\varepsilon_{ge}\right)\right)+E^{pol2}_{ge,ge}\left(\alpha\left(0\right),\alpha\left(-\varepsilon^{(A)}_{ge}\right)\right)\right]\\
&+2\frac{\left(E^{ele}_{ge}\right)^2\left(E^{ele}_{gg}-E^{ele}_{ee}\right)}{\left(\varepsilon^{(A)}_{ge}\right)^2}-\frac{E^{ele}_{ge}}{\varepsilon^{(A)}_{ge}}\left[E^{pol,1}_{(ee-gg),ge}\left(\alpha\left(\varepsilon^{(A)}_{ge}\right)\right)-E^{pol,1}_{(ee-gg),ge}\left(\alpha\left(-\varepsilon^{(A)}_{ge}\right)\right)\right]\\
&+\frac{E^{ele}_{ge}}{\varepsilon^{(A)}_{ge}}\left[E^{pol,1}_{ee,ge}\left(\alpha\left(0\right)\right)+E^{pol,1}_{gg,ge}\left(\alpha\left(0\right)\right)+2E^{env-pol,1}_{ge}\left(\alpha\left(0\right)\right)\right]\\
&-\frac{1}{2}\bar{K}\left[E^{pol,1}_{ee}\left(\beta\left(0,0\right)\right)-E^{pol,1}_{gg}\left(\beta\left(0,0\right)\right)+2E^{env-pol,1}_{ee}\left(\beta\left(0,0\right)\right)-2E^{env-pol,1}_{gg}\left(\beta\left(0,0\right)\right)\right]\\
&-\frac{1}{2}\bar{K}\left[E^{pol,1}_{ge}\left(\beta\left(\varepsilon_{ge},\varepsilon_{ge}\right)\right)-E^{pol,1}_{ge}\left(\beta\left(-\varepsilon_{ge},-\varepsilon_{ge}\right)\right)\right]\\
&+\frac{1}{2}\left(E^{ele}_{ee}-E^{ele}_{gg}\right)\left[E^{pol,1}_{ge}\left(\beta\left(\varepsilon_{ge},\varepsilon_{ge}\right)\right)+E^{pol,1}_{ge}\left(\beta\left(-\varepsilon_{ge},-\varepsilon_{ge}\right)\right)\right],
\end{aligned}
$$

where we introduced polarizability $\beta_{ij}(E_1,E_2) = 2\sum_\eta \left(\vec{\mu}^{(n)}_\eta\right)_i \left(\vec{\mu}^{(n)}_\eta\right)_j / \left(F^{(n)}_{0\eta}-E_1\right)\left(F^{(n)}_{0\eta}-E_2\right)$ and the mean Coulomb interaction $\bar{K} = \langle\sum_{n'} q_{n'}\left(0,0\right)\left(q_n\left(\eta,\eta\right)-q_n\left(0,0\right)\right)/R_{nn'}\rangle_n$ of single excited building block with all other blocks in the ground state. For small transition energy ($E \ll F^{(n)}_{0\eta}$) we can approximate the terms with $\beta$ polarizability as

$$
\begin{aligned}
\beta(E,E)-\beta(-E,-E) &\approx \frac{4}{E}\left[\alpha_{dynamic}\left(E\right)-\alpha\left(0\right)\right]\\
\beta(E,E)+\beta(-E,-E) &\approx \frac{1}{E}\left[\alpha\left(E\right)-\alpha\left(-E\right)\right]\\
\beta(0,0)\approx\beta(E,-E) &= \frac{1}{2E}\left[\alpha\left(E\right)-\alpha\left(-E\right)\right].
\end{aligned}
\tag{2}
$$

When we assume small electrostatic interaction between chromophore and its environment as compared to the chromophore transition energy, and assume small change in environment building block charges upon excitation, we can neglect terms $E^{ele}_{ge}/\varepsilon^{(A)}_{ge}$, $\bar{K}/\varepsilon^{(A)}_{ge}$, $\left(E^{ele}_{ee}-E^{ele}_{gg}\right)/\varepsilon^{(A)}_{ge}$ and we obtain the formula, which is presented in the paper.

## 1.2 Transition dipole

Applying the same approximation also to the transition dipole moment yields

$$\begin{aligned}\Delta\vec{\mu}_{GE}^{(2)} = \sum_n \vec{\mu}_{ge}^{(n)ind,2}\left(\overleftrightarrow{\alpha}_{dynamic}\left(\varepsilon_{ge}^{(A)}\right)\right) - \frac{2\left(E_{ge}^{ele}\right)^2}{\left(\varepsilon_{ge}^{(A)}\right)^2}\vec{\mu}_{ge}^{(A)} \\
+\frac{1}{2}\frac{E_{ge}^{ele}}{\varepsilon_{ge}^{(A)}}\left[\sum_n \vec{\mu}_{gg}^{(n)ind,1}\left(\overleftrightarrow{\alpha}\left(\varepsilon_{ge}^{(A)}\right)\right) - \sum_n \vec{\mu}_{ee}^{(n)ind,1}\left(\overleftrightarrow{\alpha}\left(\varepsilon_{ge}^{(A)}\right)\right)\right] \\
+\frac{1}{2}\frac{E_{ge}^{ele}}{\varepsilon_{ge}^{(A)}}\left[\sum_n \vec{\mu}_{gg}^{(n)ind,1}\left(\overleftrightarrow{\alpha}\left(-\varepsilon_{ge}^{(A)}\right)\right) - \sum_n \vec{\mu}_{ee}^{(n)ind,1}\left(\overleftrightarrow{\alpha}\left(-\varepsilon_{ge}^{(A)}\right)\right)\right] \\
+\frac{1}{4}\left[E_{ee,ee}^{pol,1}\left(\beta\left(00\right)\right) + E_{gg,gg}^{pol,1}\left(\beta\left(00\right)\right) - 2E_{gg,ee}^{pol,1}\left(\beta\left(0,0\right)\right)\right]\vec{\mu}_{ge}^{(A)} \\
+\frac{1}{2}\left(E_{ee}^{ele} - E_{gg}^{ele}\right)\sum_n\left[\vec{\mu}_{ge}^{(n)ind,1}\left(\overleftrightarrow{\beta}\left(\varepsilon_{ge}^{(A)},\varepsilon_{ge}^{(A)}\right)\right) - \sum_n \vec{\mu}_{ge}^{(n)ind,1}\left(\overleftrightarrow{\beta}\left(-\varepsilon_{ge}^{(A)},-\varepsilon_{ge}^{(A)}\right)\right)\right] \\
-\frac{1}{2}\bar{K}\sum_n\left[\vec{\mu}_{ge}^{(n)ind,1}\left(\overleftrightarrow{\beta}\left(\varepsilon_{ge}^{(A)},\varepsilon_{ge}^{(A)}\right)\right) + \vec{\mu}_{ge}^{(n)ind,1}\left(\overleftrightarrow{\beta}\left(-\varepsilon_{ge}^{(A)},-\varepsilon_{ge}^{(A)}\right)\right)\right].\end{aligned}$$

When the assumption of large chromophore transition energy is used, we obtain the formula which is presented in the paper.

## 1.3 Interaction energy

The same approach is also applied for the second order correction of homodimer inetraction energy, which reads as

$$
\begin{aligned}
J_{AB}^{(2)} \approx\ & E_{ge,ge}^{(AB)pol,2}\left(\alpha_{dynamic}\left(\varepsilon_{ge}\right)\right) + \left[E_{ee}^{(A)ele} - E_{gg}^{(A)ele}\right] \frac{\left[E_{ge,ee}^{(AB)} - E_{ge,gg}^{(AB)}\right]\left[E_{ge,gg}^{(AB)} + E_{ge,ee}^{(AB)} + 2E_{ge}^{(A)ele}\right]}{\left(\varepsilon_{ge}\right)^2} \\
& + \left(E_{gg,gg}^{(AB)} - E_{gg,ee}^{(AB)}\right) \frac{\left(E_{ge,gg}^{(AB)} + E_{ge}^{(A)ele}\right)^2}{\left(\varepsilon_{ge}\right)^2} + \left(E_{ee,ee}^{(AB)} - E_{gg,ee}^{(AB)}\right) \frac{\left(E_{ee,ge}^{(AB)} + E_{ge}^{(A)ele}\right)^2}{\left(\varepsilon_{ge}\right)^2} \\
& - V_{AB} \frac{\left[E_{ge}^{(A)ele} + E_{ee,ge}^{(AB)} + E_{ge}^{(A)ele} + E_{ge,gg}^{(AB)}\right]^2}{\left(\varepsilon_{ge}\right)^2} + \frac{E_{ge}^{(A)ele}}{\varepsilon_{ge}} \left[E_{ge,gg}^{(A)pol,1}\left(\alpha\left(\varepsilon_{ge}\right)\right) - E_{ge,ee}^{(A)pol,1}\left(\alpha\left(\varepsilon_{ge}\right)\right)\right] \\
& + \frac{E_{ge}^{(A)ele}}{\varepsilon_{ge}} \left[E_{ge,gg}^{(AB)pol,1}\left(\alpha_{dynamic}\left(\varepsilon_{ge}\right)\right) - E_{ge,ee}^{(AB)pol,1}\left(\alpha_{dynamic}\left(\varepsilon_{ge}\right)\right)\right] \\
& + 2\frac{\left[E_{ee}^{(A)ele} - E_{gg}^{(A)ele}\right]}{\varepsilon_{ge}} \left[E_{ge,ge}^{(AB),pol1}\left(\alpha_{dynamic}\left(\varepsilon_{ge}\right)\right) - E_{ge,ge}^{(AB),pol1}\left(\alpha\left(0\right)\right)\right] \\
& + \frac{E_{ge,gg}^{(AB)}}{\varepsilon_{ge}} \left[E_{ge,gg}^{(AB)pol,1}\left(\alpha\left(\varepsilon_{ge}\right)\right) - E_{ge,ee}^{(AB)pol,1}\left(\alpha\left(\varepsilon_{ge}\right)\right)\right] - \frac{E_{ge,ee}^{(AB)}}{\varepsilon_{ge}} \left[E_{ge,ee}^{(AB)pol,1}\left(\alpha\left(-\varepsilon_{ge}\right)\right) - E_{ge,gg}^{(AB)pol,1}\left(\alpha\left(-\varepsilon_{ge}\right)\right)\right] \\
& + \frac{\left[E_{ge,gg}^{(AB)} - E_{ge,ee}^{(AB)}\right]}{\varepsilon_{ge}} \left[2E_{ge}^{(A)env-pol,1}\left(\alpha\left(0\right)\right) + E_{ge,ee}^{(A)pol,1}\left(\alpha\left(0\right)\right) + E_{gg,ge}^{(A)pol,1}\left(\alpha\left(0\right)\right)\right] \\
& + \frac{\left[E_{ge,gg}^{(AB)} - E_{ge,ee}^{(AB)}\right]}{\varepsilon_{ge}} \left[E_{ge,gg}^{(AB)pol,1}\left(\alpha\left(0\right)\right) + E_{ge,ee}^{(AB)pol,1}\left(\alpha\left(0\right)\right)\right] \\
& - \frac{1}{2}V_{AB} \left[2E_{ee,gg}^{(A)pol,1}\left(\beta\left(0,0\right)\right) - E_{ee,ee}^{(A),pol1}\left(\beta\left(0,0\right)\right) - E_{gg,gg}^{(A),pol1}\left(\beta\left(0,0\right)\right)\right] \\
& + \frac{1}{2}V_{AB} \left[2E_{gg,ee}^{(AB),pol1}\left(\beta\left(0,0\right)\right) - E_{gg,gg}^{(AB)pol,1}\left(\beta\left(0,0\right)\right) - E_{ee,ee}^{(AB)pol,1}\left(\beta\left(0,0\right)\right)\right] \\
& - \frac{1}{2}\bar{K} \left[E_{ge,ge}^{(AB)pol,1}\left(\beta\left(-\varepsilon_{ge},-\varepsilon_{ge}\right)\right) + E_{ge,ge}^{(AB)pol,1}\left(\beta\left(\varepsilon_{ge},\varepsilon_{ge}\right)\right)\right] \\
& + \frac{1}{2}\left[E_{gg,ee}^{(AB)} - E_{gg,gg}^{(AB)}\right] E_{ge,ge}^{(AB),pol1}\left(\beta\left(\varepsilon_{ge},\varepsilon_{ge}\right)\right) + \frac{1}{2}\left[E_{gg,ee}^{(AB)} - E_{ee,ee}^{(AB)}\right] E_{ge,ge}^{(AB),pol1}\left(\beta\left(-\varepsilon_{ge},-\varepsilon_{ge}\right)\right).
\end{aligned}
$$

## 2 Results

In this section, we compare results for resonance coupling, transition dipole and excitation energy shift calculated with different methods. Resonance coupling dependence on the mutual distance $d$ between impurities was calculated from excited state splitting from quantum chemistry calculation $J_{QC}^{FG}$, with the quantum polarizable atom model $J_{pol}$, with the Poisson-TrEsp method $J_{PTrEsp}$, with the harmonic oscillator approximation $J_{HO}$, with the classical polarizable atom model $J_{cl}$, and also for corresponding impurity-like molecules in vacuum with quantum chemistry methods $J_{QC}^{vac}$. For calculation of resonance couplings with TrEsp method, the FG was represented as a dielectric slab and impurities as molecules in vacuum cavities. The border of the cavity around the impurities was set in the middle of C-C bond between the impurity and surrounding FG carbons. Thickness of the dielectric layer $l = 1.3$Å and its relative permitivity $\varepsilon_r = 2.2$ was obtained from fitting the quantum chemistry results. From this comparison we can see that Poisson-TrEsp cannot represent fluorographene effects on interaction energies well. The interaction energy shifts and the transition dipoles for impurities in FG were calculated with full quantum chemistry (upper index $^{QC-FG}$) calculation of FG cluster, with the quantum polarizable atom model (upper index$^{pol}$), with the harmonic oscillator approximation (upper index $^{HO}$), with the classical polarizable atom model (upper index $^{cl}$) and with quantum chemistry methods for corresponding impurity-like molecule in vacuum at the same geometry as in FG (upper

index $^{QC-vac}$).

| Parallel | | | | | | | Serial | | | | | | |
|---|---|---|---|---|---|---|---|---|---|---|---|---|---|
| $d$ [Å] | $J_{QC}^{vac}$ | $J_{QC}^{FG}$ | $J_{pol}$ | $J_{PTrEsp}$ | $J_{HO}$ | $J_{cl}$ | $d$ [Å] | $J_{QC}^{vac}$ | $J_{QC}^{FG}$ | $J_{pol}$ | $J_{PTrEsp}$ | $J_{HO}$ | $J_{cl}$ |
| 10.34 | 191 | 231 | 187 | 196 | 176 | 194 | 11.37 | 387 | 366 | 273 | 377 | 138 | 374 |
| 12.98 | 94 | 126 | 112 | 100 | 114 | 106 | 13.54 | 205 | 230 | 246 | 211 | 233 | 242 |
| 15.62 | 54 | 77 | 70 | 58 | 74 | 64 | 15.89 | 117 | 148 | 164 | 124 | 171 | 149 |
| 18.25 | 34 | 49 | 44 | 37 | 47 | 40 | 18.08 | 77 | 105 | 116 | 83 | 125 | 101 |
| | | | | | | | 20.37 | 52 | 77 | 83 | 56 | 92 | 71 |

Tab. 1: Perylene impurity homodimer interaction energy in $cm^{-1}$ together with mutual distance $d$ between impurities, for impurities with parallel and serial configuration of transition dipoles.

| Parallel | | | | | | | Serial | | | | | | |
|---|---|---|---|---|---|---|---|---|---|---|---|---|---|
| $d$ [Å] | $J_{QC}^{vac}$ | $J_{QC}^{FG}$ | $J_{pol}$ | $J_{PTrEsp}$ | $J_{HO}$ | $J_{cl}$ | $d$ [Å] | $J_{QC}^{vac}$ | $J_{QC}^{FG}$ | $J_{pol}$ | $J_{PTrEsp}$ | $J_{HO}$ | $J_{cl}$ |
| 13.78 | 82 | 180 | 171 | 92 | 202 | 133 | 10.35 | 378 | 477 | 360 | 378 | 249 | 429 |
| 16.29 | 50 | 117 | 105 | 57 | 125 | 81 | 13.00 | 175 | 270 | 272 | 186 | 285 | 242 |
| 18.82 | 33 | 79 | 68 | 37 | 81 | 53 | 15.62 | 97 | 173 | 176 | 106 | 199 | 145 |
| 21.37 | 22 | 55 | 45 | 26 | 54 | 35 | 18.25 | 60 | 118 | 118 | 66 | 138 | 94 |
| | | | | | | | 20.86 | 39 | 85 | 83 | 44 | 99 | 64 |

Tab. 2: Anthanthrene impurity homodimer interaction energy in $cm^{-1}$ together with mutual distance $d$ between impurities, for impurities with parallel and serial configuration of transition dipoles.

| Parallel | | | | | | | Serial | | | | | | |
|---|---|---|---|---|---|---|---|---|---|---|---|---|---|
| $d$ [Å] | $J_{QC}^{vac}$ | $J_{QC}^{FG}$ | $J_{pol}$ | $J_{PTrEsp}$ | $J_{HO}$ | $J_{cl}$ | $d$ [Å] | $J_{QC}^{vac}$ | $J_{QC}^{FG}$ | $J_{pol}$ | $J_{PTrEsp}$ | $J_{HO}$ | $J_{cl}$ |
| 12.99 | 154 | 231 | 180 | 160 | 182 | 172 | 11.27 | 417 | 486 | 372 | 417 | 263 | 443 |
| 15.63 | 79 | 134 | 114 | 85 | 124 | 100 | 13.48 | 228 | 307 | 313 | 240 | 317 | 291 |
| 18.26 | 47 | 85 | 74 | 51 | 83 | 63 | 15.81 | 135 | 200 | 210 | 145 | 228 | 183 |
| 20.88 | 30 | 56 | 50 | 34 | 57 | 42 | 18.03 | 90 | 144 | 151 | 98 | 169 | 126 |
| | | | | | | | 20.35 | 61 | 104 | 107 | 68 | 121 | 88 |

Tab. 3: Bisanthrene impurity homodimer interaction energy in $cm^{-1}$ together with mutual distance $d$ between impurities, for impurities with parallel and serial configuration of transition dipoles.

| Parallel | | | | | | |
|---|---|---|---|---|---|---|
| $d$ [Å] | $J_{QC}^{vac}$ | $J_{QC}^{FG}$ | $J_{pol}$ | $J_{PTrEsp}$ | $J_{HO}$ | $J_{cl}$ |
| 10.35 | 330 | 509 | 463 | 343 | 487 | 418 |
| 12.99 | 176 | 299 | 274 | 185 | 303 | 235 |
| 15.61 | 104 | 188 | 168 | 112 | 189 | 142 |
| 18.23 | 67 | 124 | 108 | 72 | 122 | 91 |

Tab. 4: Peropyrene impurity homodimer interaction energy in $cm^{-1}$ together with mutual distance $d$ between impurities, for impurities with parallel configuration of transition dipoles.

| | $\Delta E_{g\to e}^{QC-FG}$ | $\Delta E_{g\to e}^{pol}$ | $\Delta E_{g\to e}^{HO}$ | $\Delta E_{g\to e}^{cl}$ |
|---|---|---|---|---|
| Perylene[1] | -2754 | -2754 | -2736 | 447 |
| Perylene[2] | -2858 | -2860 | -2842 | 446 |
| Anthanthrene | -2352 | -2276 | -2253 | 176 |
| Bisanthrene | -1746 | -2267 | -2262 | 155 |
| Peropyrene | -2364 | -2234 | -2186 | 99 |

Tab. 5: Excitation energy difference between vacuum and fluorographene in $cm^{-1}$ obtained from quantum chemistry calculation ($\Delta E_{g\to e}^{QC}$), quantum polarizable atom model ($\Delta E_{g\to e}^{pol}$), harmonic oscillator model ($\Delta E_{g\to e}^{HO}$) and classical polarizable atom model ($\Delta E_{g\to e}^{cl}$) in the second order perturbation expansion. For perylene impurity two different orientations of the FG sheet were used, elongated in direction perpendicular to transition dipole[1] and in direction of the transition dipole[2].

| | $\mu_{g\to e}^{QC-vac}$ | $\mu_{g\to e}^{QC-FG}$ | $\mu_{g\to e}^{pol}$ | $\mu_{g\to e}^{HO}$ | $\mu_{g\to e}^{cl}$ |
|---|---|---|---|---|---|
| Perylene[1] | 2.494 | 2.691 | 2.411 | 2.212 | 2.501 |
| Perylene[2] | 2.494 | 3.093 | 2.988 | 3.043 | 2.800 |
| Anthanthrene | 2.538 | 3.705 | 3.289 | 3.422 | 2.985 |
| Bisanthrene | 2.774 | 3.462 | 3.198 | 3.172 | 3.043 |
| Peropyrene | 3.565 | 4.273 | 3.681 | 3.474 | 3.702 |

Tab. 6: Transition dipole difference in atomic units obtained from quantum chemistry calculation for impurity like molecule in vacuum ($\mu_{g\to e}^{QC-vac}$) and for impurity in fluorographene ($\mu_{g\to e}^{QC-FG}$). Quantum chemistry results are compared with results for quantum polarizable atom model ($\mu_{g\to e}^{pol}$), harmonic oscillator model ($\mu_{g\to e}^{HO}$) and classical polarizable atom model ($\mu_{g\to e}^{cl}$) of the environment in the second order perturbation expansion. For perylene impurity two different orientations of the FG sheet were used, elongated in direction perpendicular to transition dipole[1] and in direction of the transition dipole[2].

## 3 Cluster structure

Here we present individual cluster structures used for the calculation of resonance couplings between impurities in FG. These structures represent the closes distances between impurities, where differential overlap between molecular orbitals from different impurities is still negligible. The structures in distance series were constructed by shifting the impurity by single fluorograhene unit cell, for parallel arrangement of transition dipoles in direction orthogonal to the transition dipole and for serial arrangement of transition dipoles in direction of the transition dipole. The FG cluster was elongated for every distance between impurities, to keep the same number of atoms between the impurity and the borders. This procedure ensures that we have the same border effects for all clusters in the distance series.

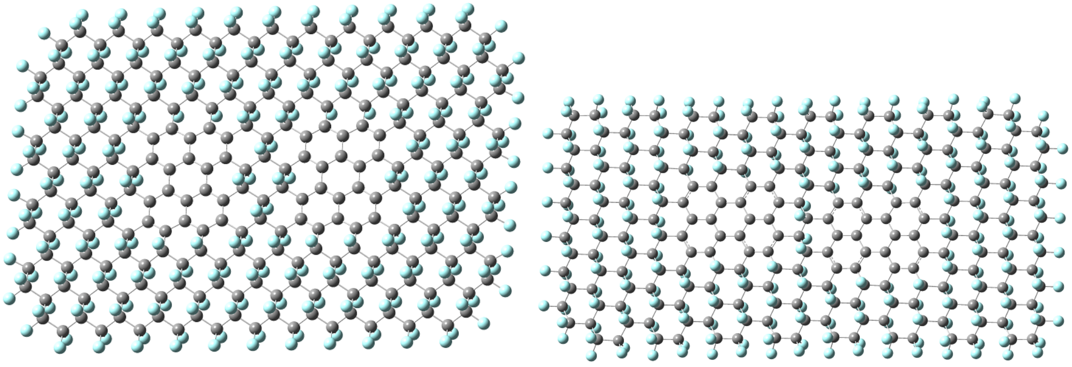

(a) (b)

Fig. 1: Perylene impurities with (a) parallel and (b) serial arrangement of transition dipoles

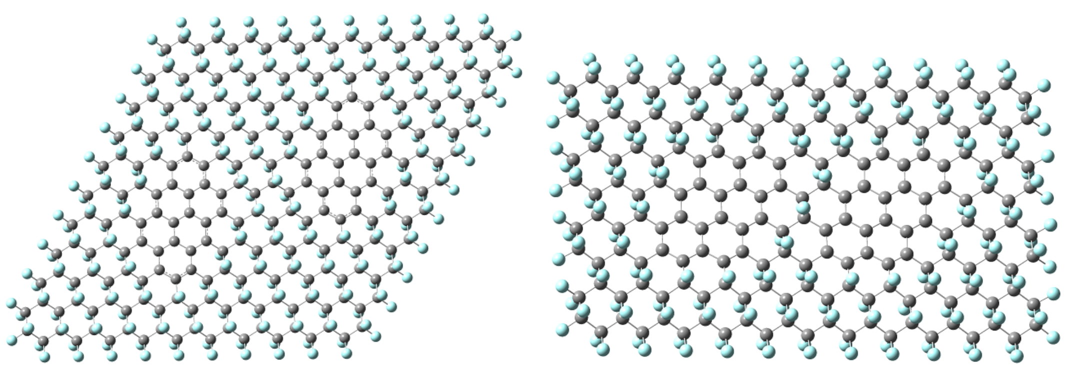

(a) (b)

Fig. 2: Anthanthrene impurities with (a) parallel and (b) serial arrangement of transition dipoles

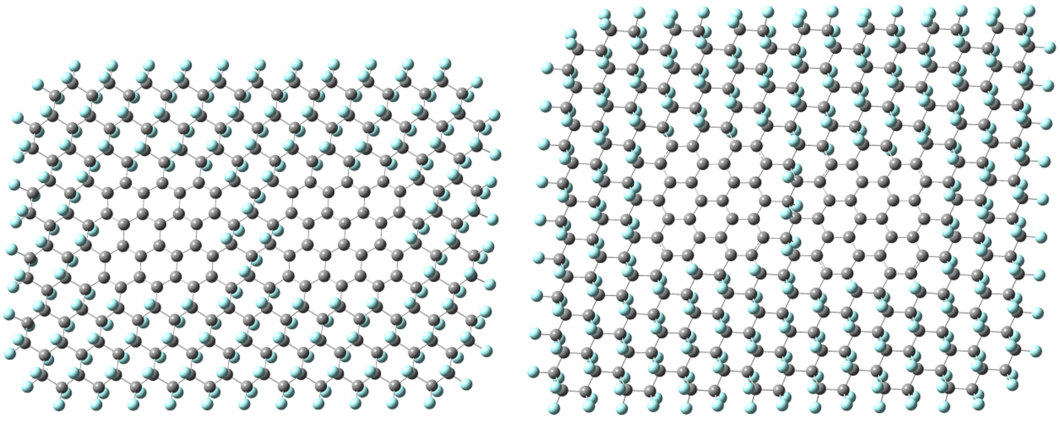

(a) (b)

Fig. 3: Bisanthrene impurities with (a) parallel and (b) serial arrangement of transition dipoles.

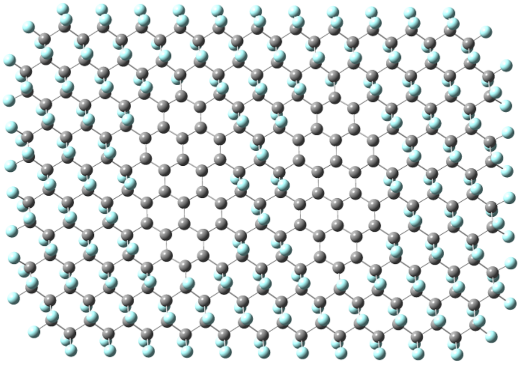

Fig. 4: Peropyrene impurities with parallel arrangement of transition dipoles.

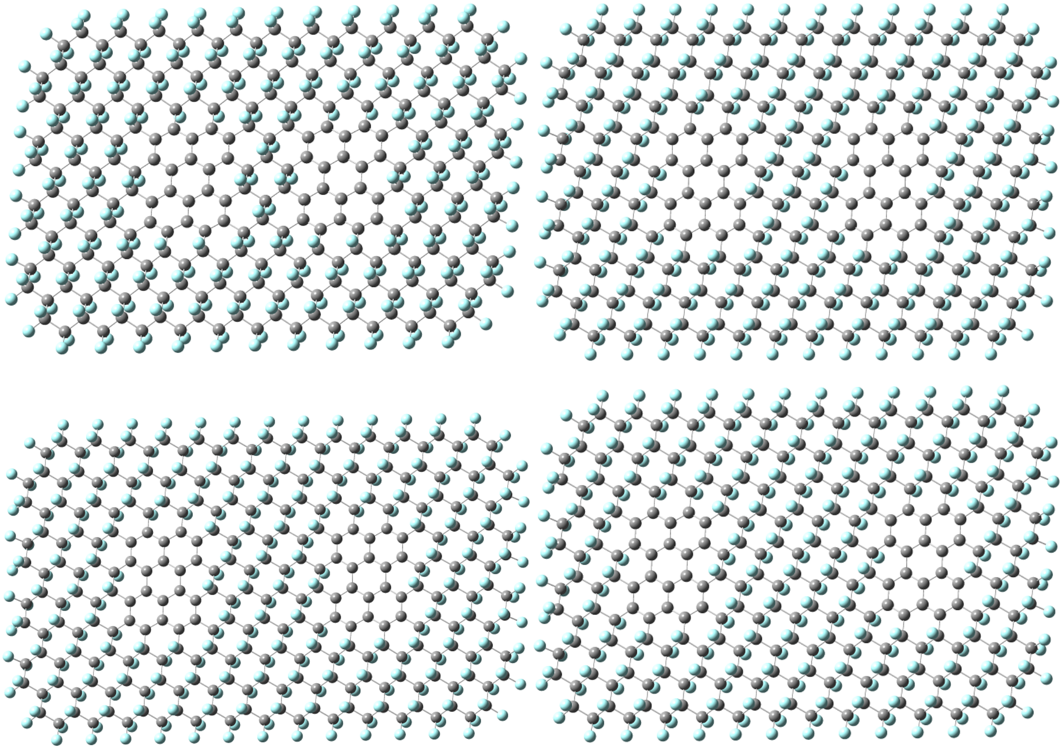

Fig. 5: Example of structures in distance series for perylene impurity in FG with parallel arrangement of transition dipole.

# 4 Charge fitting

## 4.1 Fluorographene charges

The FG ground state charges were obtaned from the RESP fitting of the ground state potential of pure FG cluster in the direction perpendicular to the FG surface for three positions around the center of the cluster, namely, in the center of the ring unit, above the fluorine atom and above the carbon atom in the direction opposite to the C-F bond (Figure 6). The potential was calculated using DFT approach

with $\omega$B97XD functional and LANL2DZ valence basis set. The distance of the points, where potential is calculated, from the FG plane was set from 0-100Å with the highest density close to the FG surface. For the charge fitting, carbons were divided into inner (inside FG sheet with single fluorine atom - upper index $^{in}$) and border carbons (at the edges of FG sheet with two connected fluorines - upper index $^{bd}$). To obtain neutral structure, the inner fluorine charge was taken the same as the inner carbon charge only with the opposite sign ($q_F^{in} = -q_C^{in}$) . For the border fluorine half of the carbon charge was used $q_F^{bd} = -q_C^{bd}/2$. For the RESP fitting, two minimal distances (2Å and 3Å) of the potential points from the nearest atom were investigated. Other option is to use Hirshfeld charges (*Theoret. Chim. Acta, 44, 129-138 (1977)*) which are widely used for charge distribution analysis in solids. When Hishfeld charges were used, inner carbon charge was set as an average charge of the six center carbons and the border carbon charge was set to an average over all border carbons. The resulting charges are shown in Table 7 and the comparison of QC and RESP potentials for two cutoff distances is presented in Figure 7. The cutoff distance of 2Å results in a slightly worse fit of the potential, and therefore the cutoff value of 3Å was used for the polarizable atom model. However, all three sets of charges provide similar results when used with polarizable atom model, only with slightly different atomic polarizabilities, which are fitted to the QC results. The RESP charges provided slightly better results then Hirshfeld charges, and they are also more physical, because they represent the correct potential of the fluorographene. Therefore the charges obtained by RESP procedure were used for production calculations in the paper.

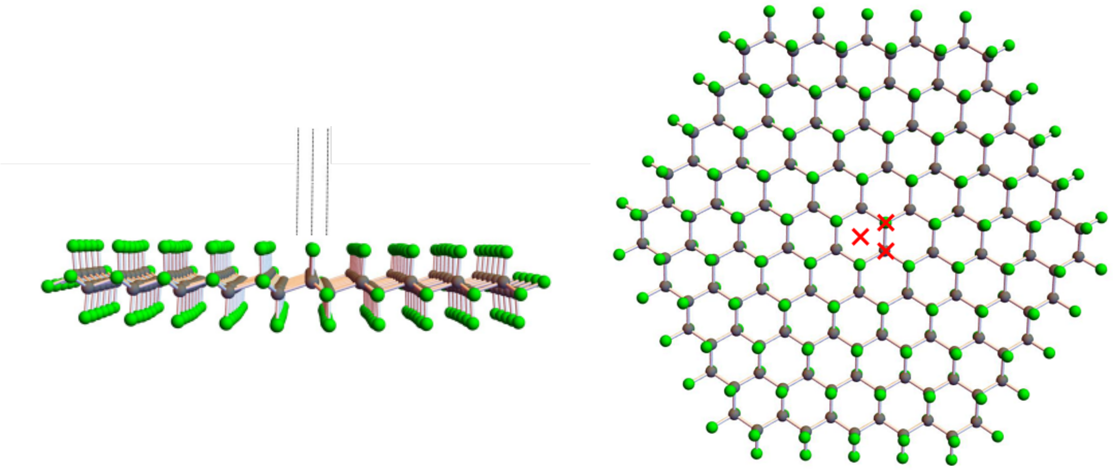

(a) Side view (b) Top view

Fig. 6: FG cluster structure and positions of points where potential for RESP fitting procedure was calculated

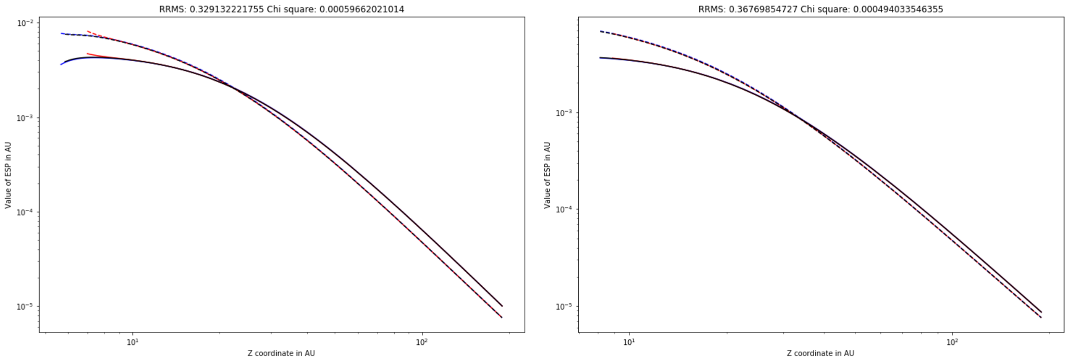


(a) Cutoff 2Å (b) Cutoff 3Å

Fig. 7: Comparison of potential from QC calculation (solid lines) and the one obtained from RESP atomic charges (dashed lines)

| | RESP 2Å cutoff | RESP 3Å cutoff | Hirshfeld |
|---|---|---|---|
| $q_C^{in}$ | -0.0608 | -0.0522 | 0.0813 |
| $q_C^{bd}$ | -0.1216 | -0.1044 | 0.1712 |
| $q_F^{in}$ | 0.0608 | 0.0522 | -0.0813 |
| $q_F^{bd}$ | 0.0608 | 0.0522 | -0.0856 |

Tab. 7: Atomic charges for FG sheet

# 5 Static polarizability

Static polarizability for six FG clusters (Figure 9) was calculated by Gaussian 09 quantum chemistry package using DFT approach with $\omega$B97XD functional and LANL2DZ valence basis set. Atomic polarizabilities were obtained from fitting of the QC results, with allowed mutual polarization of nearest neighbor bonded atoms. The comparison of static polarizability obtained from the polarizable atom model and the QC results is shown in Figure 8.

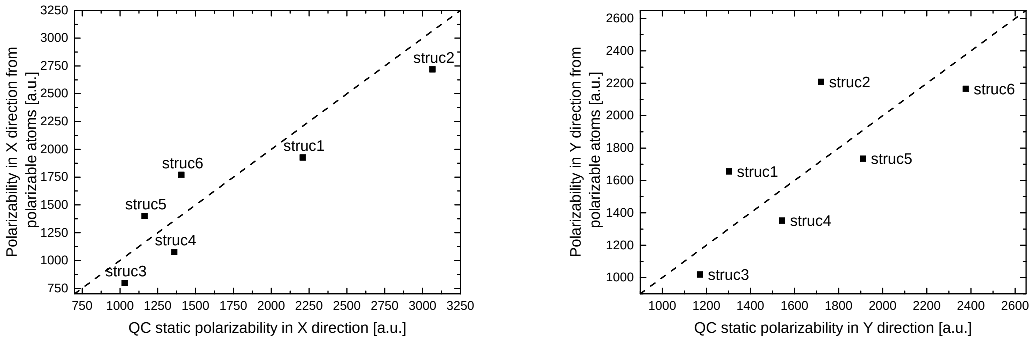


Fig. 8: Fitted static polarizabilities for testing set of pure FG clusters with C-F coarse grained polarizable atoms, where $\alpha_{\parallel}(0) = 5.10\ a.u.$ for atomic polarizability parallel to the FG surface and $\alpha_{\perp}(0) = 5.17\ a.u.$ for perpendicular to the FG surface.

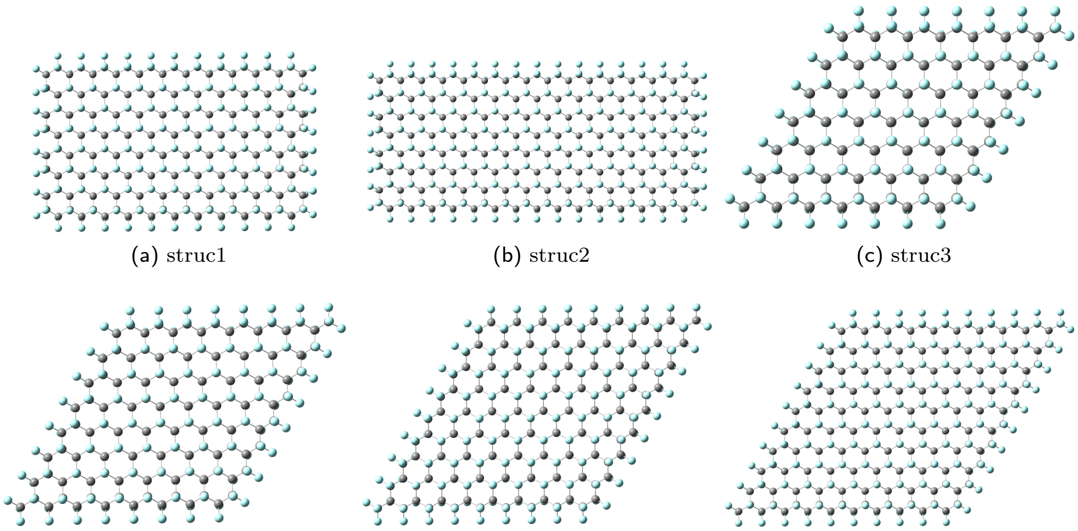

(a) struc1 (b) struc2 (c) struc3

(d) struc4 (e) struc5 (f) struc6

Fig. 9: Structures used for fitting static atomic polarizabilities
